# Supplementary material for: The fibres of the Scott map on polygon tilings are the flip equivalence classes
Source: arXiv:1601.05080 source file (2017-06-03)
Supplement: Supplementary file 3 [file macros-kapa.tex]

%{{{ MACROS
%{{{ theorem MACROS

\newtheorem{lm}{Lemma}[section]
\newtheorem*{lemma}{Lemma}
\newtheorem{prop}[lm]{Proposition}

\newtheorem*{corollary}{Corollary}
\newtheorem{cor}[lm]{Corollary}
\newtheorem{theorem}[lm]{Theorem}
\newtheorem*{thm}{Theorem}
\newtheorem{conj}[lm]{Conjecture}
%\newtheorem*{lemma}{Lemma}
%\newtheorem{remark}[lemma]{Remark}

\theoremstyle{definition}
\newtheorem{defn}[lm]{Definition}
\newtheorem*{defini}{Definition}
\newtheorem*{notation}{Notation}
\newtheorem{claim}[lm]{Claim}
%\newtheorem{bsp}{Beispiel}
\newtheorem{ex}[lm]{Example}
\newtheorem*{exas}{Beispiele}
\newtheorem*{rem}{Remark}
\newtheorem{remark}[lm]{Remark}
\newtheorem{qu}{Question}
\newtheorem*{obs}{Observations}
\newtheorem{para}[lm]{}
\newtheorem{idea}[lm]{Idea}

\newcommand{\mdef}{\refstepcounter{lm}\medskip\noindent{\bf (\thelm) } }


%}}}
%{{{ karins
%%%%%%%%%%%%% karins additions:

\renewcommand{\Re}{{\mathbb R}}  %% renamed reals!

\newcommand{\RR}{\operatorname{\mathbb{R}}\nolimits}
\newcommand{\Z}{\operatorname{\mathbb{Z}}\nolimits}


\newcommand{\ttt}{\tau}  %% maxl cycle in S_n
\newcommand{\Anii}{A_{n,(i,i+1)}}
\newcommand{\Scott}{{\boldsymbol\sigma}}  %% hook for Scott map (not yet globally used)
\newcommand{\Scottt}{{\protect\overrightarrow{\boldsymbol\sigma}}\!}  % trying out a new symbol for Scottt

\def\commentK#1{\textcolor{blue}{ [\texttt{#1}]}}  %commentK, green (without [] 

\newcommand{\qqq}[1]{\footnote{\textcolor{blue}{#1}}}
\newcommand{\ignore}[1]{}
\newcommand{\rank}{order}
\newcommand{\triangular}{flip}
\newcommand{\triangulation}{flip}
\newcommand{\tiling}{strand}
\newcommand{\regular}{regular}
%
\newcommand{\ul}[1]{\underline{#1}}
\newcommand{\Power}{{\mathcal P}}
\newcommand{\gam}{\gamma}
\newcommand{\mdefn}[1]{\begin{defn} #1 \end{defn}} %% shortcut

\newcommand{\mat}[1]{\left( \begin{array}{#1} }
\newcommand{\tam}{\end{array} \right) }

\newcommand\scalemath[2]{\scalebox{#1}{\mbox{\ensuremath{\displaystyle #2}}}}

%}}}
%{{{ more

\newcommand{\SM}{(S,M)} %%  
\newcommand{\ASM}{A\SM} %%  
\newcommand{\del}{\Delta} % set of ideal triangs
\newcommand{\FST}{\cite{FominShapiroThurston}}

\newcommand{\N}{{\mathbb N}}
\newcommand{\pp}{p} 
\newcommand{\profile}{profile}
\newcommand{\oprofile}{ordered profile}
\newcommand{\Md}{M_\partial}  %% bdry subset of M 

\newcommand{\SMP}{(S,\underline{m},\pp)}

\newcommand{\te}[1]{[ #1 ]_{\Delta}}  %% triangular equiv
\newcommand{\ASD}{alternating strand diagram}

\newcommand{\Sym}{\Sigma}  %% set of perms of n is \Sym_n

\newcommand{\srep}{stellar-replacement}% %% 
\newcommand{\Gst}{{\mathsf G}}% %% G map = stellar-replacement map

\newcommand{\pgr}{\gamma}
\newcommand{\Pb}{{\mathsf {Pl}}} %  plabic hook
\newcommand{\Pbr}{{\mathsf {Pb}}} % reduced plabic hook
\newcommand{\Pf}{{\mathsf {Pf}}}  % fully reduced plabic hook
\newcommand{\Pfim}{{\mathsf {Pt}}}  % fully reduced plabic hook
\newcommand{\bouquet}{bouquet} 
\newcommand{\Gprime}{\Gst'}% %% G' map = candidate for inverse to stellar-replacement map
\newcommand{\mm}{{\mathsf m}}  %% medial map hook

%}}}
%%%  pauls
\newcommand{\ppm}[1]{\textcolor{green}{#1}}
\newcommand{\kb}[1]{\textcolor{orange}{#1}}
\newcommand{\kub}[1]{\textcolor{blue}{#1}}
\newcommand{\face}{face}  %% face or region?


%%% figure logistics %%%
\newcommand{\fd}{./figd/}  %% point to the default Figure Directory
\newcommand{\figgdir}{./fig/} %% point to the alternate figure directory
\newcommand{\figg}[2]{\includegraphics[width=#1cm]{\figgdir #2}}
\newcommand{\includegraphicss}[2][]{\includegraphics[#1]{\fd #2}}
    %%% this is a version of includegraphics that looks for files in 
    %%% the default fig dir.

\newcommand{\pfig}[2]{\begin{figure}
    \includegraphics[width=5cm]{./fignew/#1.eps}
    \caption{#2 \label{fig:#1}}
  \end{figure}
}

%}}}


%{{{ Local vars

% Local Variables:
% mode: LaTeX
% folded-file: t
% End:

%}}}
