# Supplementary material for: The fibres of the Scott map on polygon tilings are the flip equivalence classes
Source: arXiv:1601.05080 source file (2017-06-03)
Supplement: Supplementary file 4 [file macros-ppm.tex]

% $Id: macros-ppm.tex,v 1.1 $

\newcommand{\beq}{\begin{equation}}
\newcommand{\eq}{\end{equation}}

%{{{ Local Variables

% Local Variables:
% folded-file: t
% End:

%}}}
